# Supplementary material for: Measuring Five Accountable Talk Moves to Improve Instruction at Scale
Source: arXiv:2311.10749 source file (2023-11-02)
Supplement: Supplementary file 1 [file data_appendix.tex]

\begin{table}[]
\begin{tabular}{l|ll}
Number of examples                                     & \multicolumn{2}{l}{2503} \\
Number of labels                                       & \multicolumn{2}{l}{9}    \\
Number of unique raters                                & \multicolumn{2}{l}{6}    \\
Number of raters / examples                            & \multicolumn{2}{l}{2}    \\
\multirow{4}{*}{Labels per example}                    & 1:         & 50\%        \\
                                                       & 2:         & 35\%        \\
                                                       & 3:         & 10\%        \\
                                                       & 4+:        & 5\%         \\
\begin{tabular}[c]{@{}l@{}}Examples with both raters \\ agreeing on at least 1 label\end{tabular} & \multicolumn{2}{l}{63\%}
\end{tabular}
\caption{Summary statistics of our data}
\label{tab:data_profile}
\end{table}

\begin{table}
\footnotesize

\begin{tabular}{l|c}
Label & \% examples with label \\ \hline

Adding on & 25\% \\ 
Connecting & 4\% \\ 
Eliciting & 17\% \\
Probing & 13\% \\ 
Revoicing & 11\% \\ 
Model utterance & 9\% \\ 
Poor transcription quality & 5\% \\
Off task & 28\% \\ 
No talk moves found & 60\% \\ 
\end{tabular}

    \caption{Distribution of our labels (with one or more annotators selecting label)}
    \label{tab:label_dist}  

\end{table} 

\begin{table*}[]
\centering
\resizebox{\textwidth}{!}{%
\begin{tabular}{lllllllll}
\hline
                           & Annotator 1 & Annotator 2 & Annotator 3 & Annotator 4 & Annotator 5 & Annotator 6 & Average & Range \\ \hline
Adding on                  & 82\%        & 69\%        & 83\%        & 82\%        & 85\%        & 86\%        & 81\%    & 17    \\ \hline
Connecting                 & 98\%        & 98\%        & 95\%        & 96\%        & 97\%        & 98\%        & 97\%    & 3     \\ \hline
Eliciting                  & 93\%        & 90\%        & 89\%        & 88\%        & 88\%        & 90\%        & 90\%    & 5     \\ \hline
Probing                    & 94\%        & 94\%        & 85\%        & 88\%        & 92\%        & 91\%        & 91\%    & 9     \\ \hline
Revoicing                  & 94\%        & 95\%        & 92\%        & 93\%        & 91\%        & 92\%        & 93\%    & 4     \\ \hline
Model utterance           & 91\%        & 94\%        & 86\%        & 92\%        & 94\%        & 95\%        & 92\%    & 8     \\ \hline
Poor transcription quality & 98\%        & 98\%        & 91\%        & 96\%        & 96\%        & 96\%        & 96\%    & 7     \\ \hline
Off task        & 87\%        & 89\%        & 89\%        & 89\%        & 86\%        & 86\%        & 88\%    & 3     \\ \hline
No talk moves found        & 69\%        & 64\%        & 73\%        & 73\%        & 74\%        & 70\%        & 70\%    & 10    \\ \hline
\end{tabular}%
}
\caption{Annotator agreement measured by percentage annotator selected the same label with every other annotator}
\label{tab:agreement}
\end{table*}
